# Supplementary material for: Exact exchange-correlation kernels for optical spectra of model systems
Source: arXiv:1812.05512 source file (2019-03-21)
Supplement: Supplementary file 1 [file Supplemental_Material.pdf]

# Exact exchange-correlation kernels for optical spectra of model systems (Supplemental Material)

M. T. Entwistle and R. W. Godby
*Department of Physics, University of York, and European Theoretical Spectroscopy Facility, Heslington, York YO10 5DD, United Kingdom*

(Dated: March 21, 2019)

This document provides details on the model systems and our calculations as detailed in [URL to LZ15774 will be inserted by publisher].

## SUM RULE

The exact $f_{\rm xc}$ satisfies the zero-force sum rule [1, 2],

$$\int f_{\rm xc}(x, x', \omega)\ \partial_{x'} n_0(x')\ dx' = \partial_x v_{{\rm xc},0}(x), \tag{1}$$

where $n_0$ is the ground-state density and $v_{{\rm xc},0}$ is the ground-state xc potential. As well as giving the correct absorption spectrum from the exact $\chi_0$, we check that the $f_{\rm xc}$ for each model system satisfies this sum rule.

## SYSTEM 1 (TWO-ELECTRON HARMONIC WELL)

The external potential is:

$$V_{\rm ext}(x) = \frac{1}{2}\omega_0^2 x^2, \tag{2}$$

where $\omega_0 = 0.25$ a.u. We calculate the first twenty many-electron eigenstates and the first twenty Kohn-Sham orbitals, to obtain converged results for $\chi$ and $\chi_0$ respectively. The grid spacing is $\delta x = 0.08$ a.u. and we have replaced the positive infinitesimal $\eta$ with 0.005 to broaden the absorption peaks for ease of viewing. The calculated excitation energies are given in Table I. We verify that the exact $f_{\rm xc}$ obtained is correct by checking that it satisfies Eq. 1 (Fig. 1(a)).

TABLE I: The excitation energies of the harmonic well system. All energies are in a.u. with estimated errors $\pm 1$ in the last decimal place.

| | | | |
|---|---|---|---|
| 0.2500 | 0.9378 | 1.2500 | 1.6713 |
| 0.4616 | 0.9616 | 1.4213 | 1.6878 |
| 0.5000 | 1.0000 | 1.4378 | 1.7116 |
| 0.7116 | 1.1878 | 1.4616 | 1.7500 |
| 0.7500 | 1.2116 | 1.5000 | |

## SYSTEM 2 (TWO-ELECTRON ATOM)

The external potential is:

$$V_{\rm ext}(x) = -\frac{1}{|ax| + 1}, \tag{3}$$

where $a = \frac{1}{20}$. We calculate the first twenty many-electron eigenstates and the first twenty Kohn-Sham orbitals, to obtain converged results for $\chi$ and $\chi_0$ respectively. The grid spacing is $\delta x = 0.12$ a.u. and we have replaced the positive infinitesimal $\eta$ with 0.002 to broaden the absorption peaks for ease of viewing. The calculated excitation energies are given in Table II. We verify that the exact $f_{\rm xc}$ obtained is correct by checking that it satisfies Eq. 1 (Fig. 1(b)).

[1] G. Vignale, Physics Letters A **209**, 206 (1995).
[2] M. Thiele and S. Kümmel, Phys. Rev. A **80**, 012514 (2009).

TABLE II: The excitation energies of the atom-like system. All energies are in a.u. with estimated errors ±1 in the last decimal place.

| | | | |
|---|---|---|---|
| 0.0448 | 0.1752 | 0.2418 | 0.2913 |
| 0.0859 | 0.1975 | 0.2584 | 0.2925 |
| 0.1187 | 0.2000 | 0.2590 | 0.3019 |
| 0.1448 | 0.2213 | 0.2655 | 0.3060 |
| 0.1504 | 0.2312 | 0.2761 | |

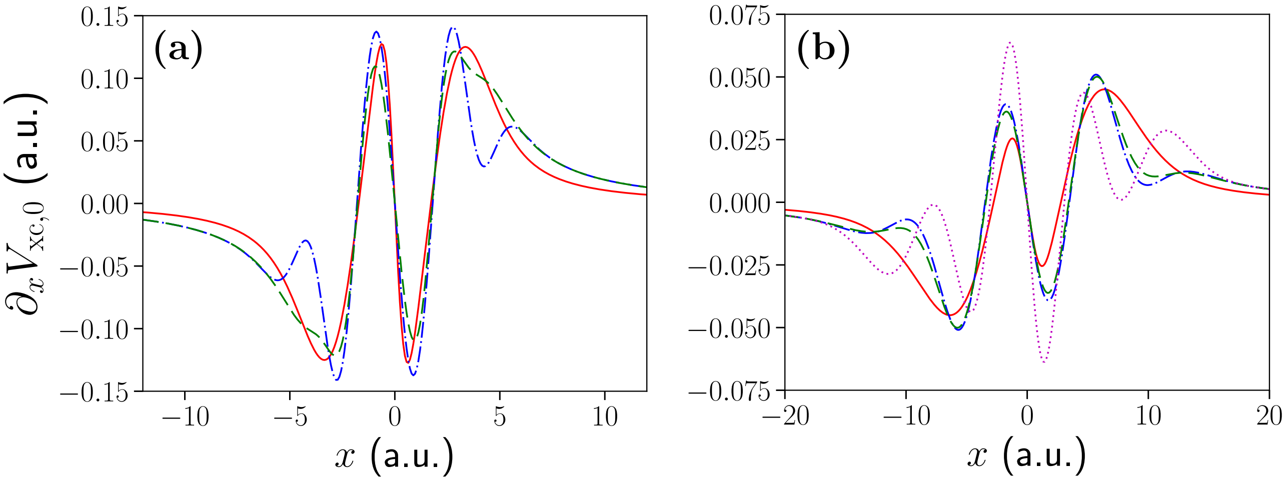


FIG. 1: We confirm the exact $f_{\mathrm{xc}}$ obtained for each system satisfies the sum rule (Eq. 1). The RHS of the equation is obtained through direct differentiation of the exact ground-state xc potential (solid red in both plots): (a) For the harmonic well system, we evaluate the LHS of the equation at $\omega = 0$ (dotted-dashed blue) and at the first excitation $\omega = \omega_0$ (dashed green), both of which should be equal to the RHS if the sum rule is satisfied. (b) For the atom-like system, we evaluate the LHS of the equation at $\omega = 0$ (dotted-dashed blue), at the first excitation $\omega = 0.0448$ (dashed green) and at the third excitation $\omega = 0.1187$ (dotted magenta), all of which should be equal to the RHS if the sum rule is satisfied. While there are discrepancies between the sets of curves in both plots, it is important to note that these discrepancies are much smaller in magnitude than $f_{\mathrm{xc}}$ is (Fig. 2 and Fig. 6 in the main paper). They can therefore be attributed to small numerical errors in $f_{\mathrm{xc}}$.
